# Supplementary material for: Disentanglement of Correlated Factors via Hausdorff Factorized Support
Source: arXiv:2210.07347 source file (2023-02-25)
Supplement: Supplementary file 1 [file supplementary_full_tables.tex]

\begin{table*}[t]
\caption{shapes3d}\centering\resizebox{1\textwidth}{!}{
\begin{tabular}{|l|l|l|l|l|l|l|l|l|l|l|l|l|}
\toprule
Method & No Corr. & Pair: 1 [V1, $\sigma$ = 0.1] & Pair: 1 [V2, $\sigma$ = 0.1] & Pair: 1 [V3, $\sigma$ = 0.1] & Pairs: 2 [V1, $\sigma$ = 0.4] & Pairs: 2 [V2, $\sigma$ = 0.4] & Pairs: 2 [V1, $\sigma$ = 0.1] & Pairs: 2 [V2, $\sigma$ = 0.1] & Pairs: 3 [V1, $\sigma$ = 0.1] & Pairs: 3 [V2, $\sigma$ = 0.1] & Conf. [V1, $\sigma$ = 0.2] & Conf. [V2, $\sigma$ = 0.2]\\
\hline
$\beta$-VAE & 70.7 [65.2, 75.4] & 55.9 [53.8, 59.0] & 71.6 [60.9, 72.5] & 66.1 [62.8, 67.0] & 68.5 [56.8, 76.9] & 71.5 [68.1, 75.1] & 58.7 [57.1, 62.9] & 55.6 [45.8, 57.2] & 37.1 [32.3, 38.9] & 40.0 [33.8, 47.5] & 46.8 [42.0, 50.7] & 38.0 [35.0, 38.6]\\
\hline
$\beta$-VAE + H-FSL, $\beta = 0$ & 78.3 [75.1, 83.6] & 56.4 [46.6, 60.2] & 77.8 [74.4, 78.8] & 68.1 [61.2, 69.4] & 73.9 [65.5, 80.0] & 76.7 [69.7, 81.2] & 62.6 [61.2, 64.3] & 56.0 [41.0, 57.4] & 47.5 [38.0, 49.1] & 41.1 [31.7, 42.7] & 51.3 [46.2, 52.5] & 46.2 [36.3, 47.5]\\
$\beta$-VAE + H-FSL, fixed $\beta = 4$ & 81.2 [76.0, 97.2] & 64.6 [57.1, 68.0] & 80.7 [78.5, 81.8] & \blue{\textbf{76.1 [72.2, 79.5]}} & \blue{\textbf{89.1 [78.2, 98.5]}} & 81.3 [75.0, 86.2] & 63.7 [61.0, 65.4] & \blue{\textbf{67.6 [62.4, 69.3]}} & 44.9 [38.9, 45.6] & 52.0 [48.7, 54.5] & 51.7 [50.0, 57.5] & 62.8 [60.2, 64.5]\\
$\beta$-VAE + H-FSL, optimal $\beta, \gamma$ & \blue{\textbf{91.2 [75.8, 100.0]}} & \blue{\textbf{67.3 [59.5, 72.3]}} & \blue{\textbf{80.9 [76.4, 81.4]}} & \blue{\textbf{76.1 [72.2, 79.5]}} & \blue{\textbf{89.1 [78.2, 98.5]}} & \blue{\textbf{83.3 [79.0, 86.5]}} & 65.5 [62.0, 66.6] & \blue{\textbf{67.6 [62.4, 69.3]}} & \blue{\textbf{47.9 [44.0, 50.8]}} & 52.0 [48.7, 54.5] & \blue{\textbf{59.7 [58.6, 62.1]}} & \blue{\textbf{63.5 [61.2, 65.5]}}\\
\hline
$\beta$-TCVAE & 77.1 [76.6, 78.3] & 62.0 [56.6, 64.5] & 71.1 [65.5, 72.5] & 69.8 [67.3, 70.8] & 75.8 [73.0, 79.1] & 75.2 [69.0, 75.9] & \blue{\textbf{65.7 [62.9, 70.0]}} & 63.8 [59.1, 65.1] & 47.3 [36.7, 50.0] & \blue{\textbf{58.1 [56.2, 61.1]}} & 55.9 [52.7, 59.9] & 49.9 [45.8, 55.9]\\
FactorVAE & 66.1 [51.2, 69.1] & 52.2 [44.7, 54.8] & 70.8 [70.5, 71.2] & 65.9 [64.2, 67.8] & 70.2 [64.8, 75.0] & 71.2 [63.0, 77.7] & 62.0 [60.7, 64.5] & 57.2 [55.9, 62.0] & 46.8 [40.8, 49.0] & 40.2 [35.2, 44.6] & 39.2 [34.2, 47.8] & 31.6 [27.9, 35.1]\\
AnnealedVAE & 62.2 [60.7, 63.2] & 39.6 [29.6, 41.6] & 57.2 [49.5, 59.3] & 56.3 [53.0, 57.2] & 60.4 [59.3, 64.9] & 48.5 [39.7, 49.1] & 50.9 [46.0, 52.9] & 31.6 [26.9, 34.1] & 33.6 [31.0, 38.0] & 30.2 [27.1, 30.8] & 26.2 [22.0, 26.8] & 23.0 [20.1, 25.9]\\
\bottomrule
\end{tabular}}
\end{table*}

\begin{table*}[t]
\caption{mpi3d}\centering\resizebox{1\textwidth}{!}{
\begin{tabular}{|l|l|l|l|l|l|l|l|l|l|l|l|l|}
\toprule
Method & No Corr. & Pair: 1 [V1, $\sigma$ = 0.1] & Pair: 1 [V2, $\sigma$ = 0.1] & Pair: 1 [V3, $\sigma$ = 0.1] & Pairs: 2 [V1, $\sigma$ = 0.4] & Pairs: 2 [V2, $\sigma$ = 0.4] & Pairs: 2 [V1, $\sigma$ = 0.1] & Pairs: 2 [V2, $\sigma$ = 0.1] & Pairs: 3 [V1, $\sigma$ = 0.1] & Pairs: 3 [V2, $\sigma$ = 0.1] & Conf. [V1, $\sigma$ = 0.2] & Conf. [V2, $\sigma$ = 0.2]\\
\hline
$\beta$-VAE & 25.6 [24.7, 26.1] & 15.7 [13.9, 17.0] & 20.5 [17.7, 20.9] & 23.5 [22.5, 24.4] & 23.6 [21.3, 24.7] & 24.8 [24.5, 25.9] & 21.2 [19.5, 21.7] & 23.6 [22.6, 24.3] & 11.6 [11.1, 11.7] & 11.1 [10.9, 11.3] & 15.1 [14.5, 15.8] & 11.8 [10.0, 12.7]\\
\hline
$\beta$-VAE + H-FSL, $\beta = 0$ & \blue{\textbf{32.8 [30.0, 34.3]}} & 20.7 [19.5, 21.2] & \blue{\textbf{28.4 [26.5, 29.5]}} & \blue{\textbf{26.9 [24.7, 28.0]}} & \blue{\textbf{30.1 [29.7, 31.0]}} & \blue{\textbf{30.2 [29.5, 30.5]}} & \blue{\textbf{25.6 [24.0, 26.2]}} & \blue{\textbf{28.0 [27.4, 28.2]}} & \blue{\textbf{14.3 [13.1, 14.8]}} & \blue{\textbf{19.0 [17.8, 19.3]}} & \blue{\textbf{18.9 [14.4, 19.2]}} & \blue{\textbf{16.1 [15.0, 16.6]}}\\
$\beta$-VAE + H-FSL, optimal $\beta, \gamma$ & \blue{\textbf{32.8 [30.0, 34.3]}} & 20.7 [19.5, 21.2] & \blue{\textbf{28.4 [26.5, 29.5]}} & \blue{\textbf{26.9 [24.7, 28.0]}} & \blue{\textbf{30.1 [29.7, 31.0]}} & \blue{\textbf{30.2 [29.5, 30.5]}} & \blue{\textbf{25.6 [24.0, 26.2]}} & \blue{\textbf{28.0 [27.4, 28.2]}} & \blue{\textbf{14.3 [13.1, 14.8]}} & \blue{\textbf{19.0 [17.8, 19.3]}} & \blue{\textbf{18.9 [14.4, 19.2]}} & \blue{\textbf{16.1 [15.0, 16.6]}}\\
\hline
$\beta$-TCVAE & 26.6 [26.0, 27.4] & \blue{\textbf{21.6 [20.4, 23.8]}} & 20.7 [20.4, 21.3] & 23.7 [23.5, 24.2] & 25.6 [25.1, 25.9] & 25.6 [25.4, 26.2] & 21.6 [19.9, 23.2] & 23.3 [21.9, 23.8] & 11.4 [10.3, 12.6] & 16.5 [15.4, 18.2] & 16.7 [16.0, 17.1] & 14.2 [13.4, 15.4]\\
FactorVAE & 26.0 [24.8, 27.5] & 20.1 [15.5, 22.7] & 21.9 [20.1, 23.9] & 24.6 [23.8, 26.2] & 25.0 [24.0, 25.9] & 27.8 [27.2, 29.2] & 21.9 [18.6, 24.0] & 21.6 [17.6, 24.4] & 10.9 [10.7, 11.9] & 15.4 [14.8, 16.4] & 15.5 [15.0, 16.5] & 13.6 [12.8, 13.9]\\
AnnealedVAE & 11.8 [10.8, 12.4] & 10.8 [9.6, 11.9] & 11.7 [10.4, 12.9] & 10.6 [10.3, 11.9] & 12.9 [11.0, 14.8] & 11.8 [11.6, 12.1] & 10.8 [9.8, 11.6] & 12.5 [10.1, 13.5] & 11.6 [10.6, 12.2] & 10.1 [9.8, 11.0] & 13.3 [11.4, 13.8] & 13.4 [12.8, 13.9]\\
\bottomrule
\end{tabular}}
\end{table*}

\begin{table*}[t]
\caption{dsprites}\centering\resizebox{1\textwidth}{!}{
\begin{tabular}{|l|l|l|l|l|l|l|l|l|}
\toprule
Method & No Corr. & Pair: 1 [V1, $\sigma$ = 0.1] & Pair: 1 [V2, $\sigma$ = 0.1] & Pair: 1 [V3, $\sigma$ = 0.1] & Pairs: 2 [V1, $\sigma$ = 0.4] & Pairs: 2 [V1, $\sigma$ = 0.1] & Conf. [V1, $\sigma$ = 0.2] & Conf. [V2, $\sigma$ = 0.2]\\
\hline
$\beta$-VAE & 32.2 \gs{[25.3, 37.9]} & 17.9 \gs{[10.4, 23.0]} & 9.5 \gs{[7.9, 10.3]} & 13.5 \gs{[9.8, 16.1]} & 20.5 \gs{[18.7, 27.6]} & 7.5 \gs{[6.7, 8.3]} & 14.0 \gs{[10.4, 18.5]} & 11.4 \gs{[9.9, 13.9]}\\
\hline
$\beta$-VAE + H-FSL, $\beta = 0$ & 34.9 \gs{[27.4, 36.0]} & 22.7 \gs{[14.4, 25.6]} & 13.6 \gs{[7.6, 16.7]} & 23.3 \gs{[13.8, 28.4]} & 24.1 \gs{[13.3, 30.3]} & 11.9 \gs{[9.7, 13.8]} & 15.8 \gs{[5.4, 18.9]} & 15.1 \gs{[11.0, 16.0]}\\
$\beta$-VAE + H-FSL, fixed $\beta = 2$ & 47.2 \gs{[27.4, 47.4]} & 30.6 \gs{[24.4, 31.6]} & 16.2 \gs{[15.4, 18.4]} & 25.1 \gs{[19.3, 30.8]} & 29.9 \gs{[24.2, 33.4]} & 16.8 \gs{[9.8, 17.5]} & 22.1 \gs{[17.7, 24.4]} & 13.4 \gs{[10.1, 15.6]}\\
$\beta$-VAE + H-FSL, optimal $\beta, \gamma$ & \blue{\textbf{49.9 \gs{[30.0, 50.4]}}} & 32.9 \gs{[21.3, 39.0]} & 19.7 \gs{[17.0, 21.1]} & \blue{\textbf{37.5 \gs{[25.9, 39.1]}}} & \blue{\textbf{38.2 \gs{[21.9, 41.7]}}} & \blue{\textbf{17.3 \gs{[6.0, 19.6]}}} & 22.1 \gs{[17.7, 24.4]} & 15.8 \gs{[12.3, 16.7]}\\
\hline
$\beta$-TCVAE & 30.9 \gs{[28.9, 35.2]} & 35.1 \gs{[32.3, 38.4]} & \blue{\textbf{24.0 \gs{[23.6, 24.4]}}} & 25.0 \gs{[19.0, 30.9]} & 30.2 \gs{[27.9, 42.2]} & 11.4 \gs{[7.6, 13.6]} & \blue{\textbf{29.4 \gs{[28.7, 30.9]}}} & \blue{\textbf{20.9 \gs{[17.5, 23.6]}}}\\
FactorVAE & 25.7 \gs{[20.9, 30.9]} & 22.6 \gs{[20.8, 25.4]} & 15.1 \gs{[11.9, 16.3]} & 21.2 \gs{[19.2, 24.6]} & 21.2 \gs{[13.5, 22.9]} & 13.4 \gs{[12.4, 15.0]} & 18.3 \gs{[17.5, 19.2]} & 14.7 \gs{[13.5, 15.3]}\\
AnnealedVAE & 39.4 \gs{[38.7, 40.0]} & \blue{\textbf{40.8 \gs{[39.4, 41.3]}}} & 14.8 \gs{[14.3, 15.9]} & 29.0 \gs{[26.6, 29.9]} & 30.3 \gs{[28.3, 31.4]} & 8.5 \gs{[6.9, 10.3]} & 19.1 \gs{[18.2, 19.2]} & 14.3 \gs{[14.1, 14.5]}\\
\bottomrule
\end{tabular}}
\end{table*}
